# Supplementary material for: Origami in N dimensions: How feed-forward networks manufacture linear separability
Source: arXiv:2203.11355 ancillary file (2022-03-21)

S1-pokernet-100-100-tuning-layer1

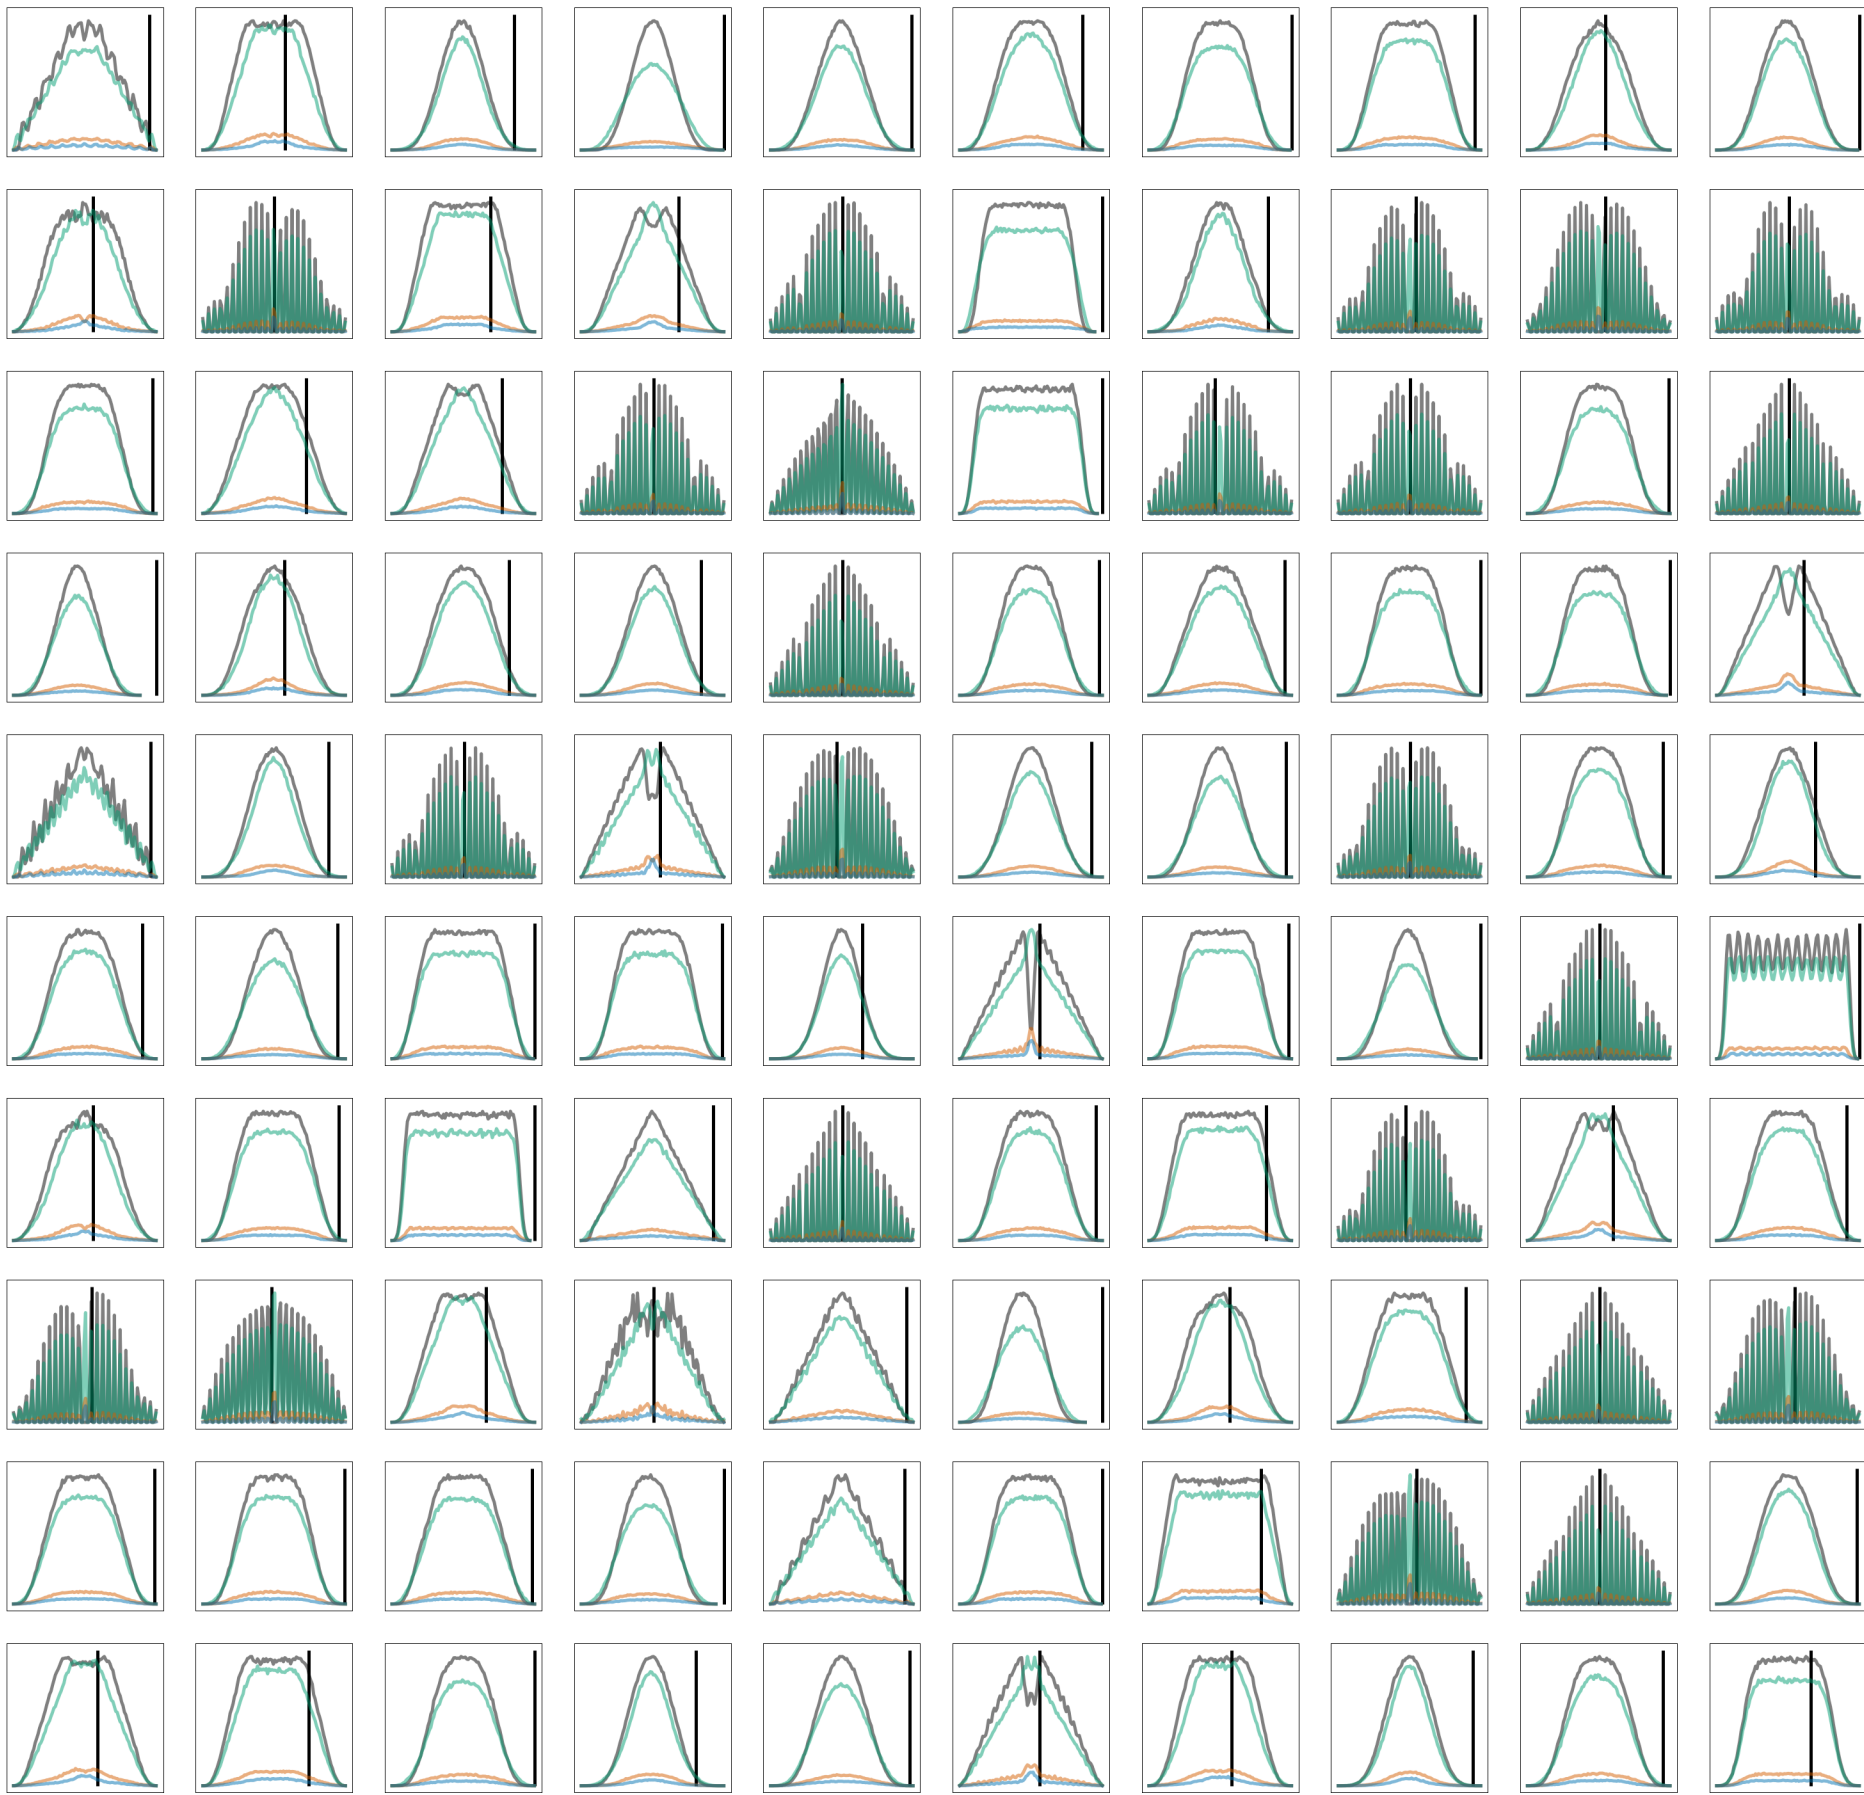

S2-pokernet-100-100-tuning-layer2

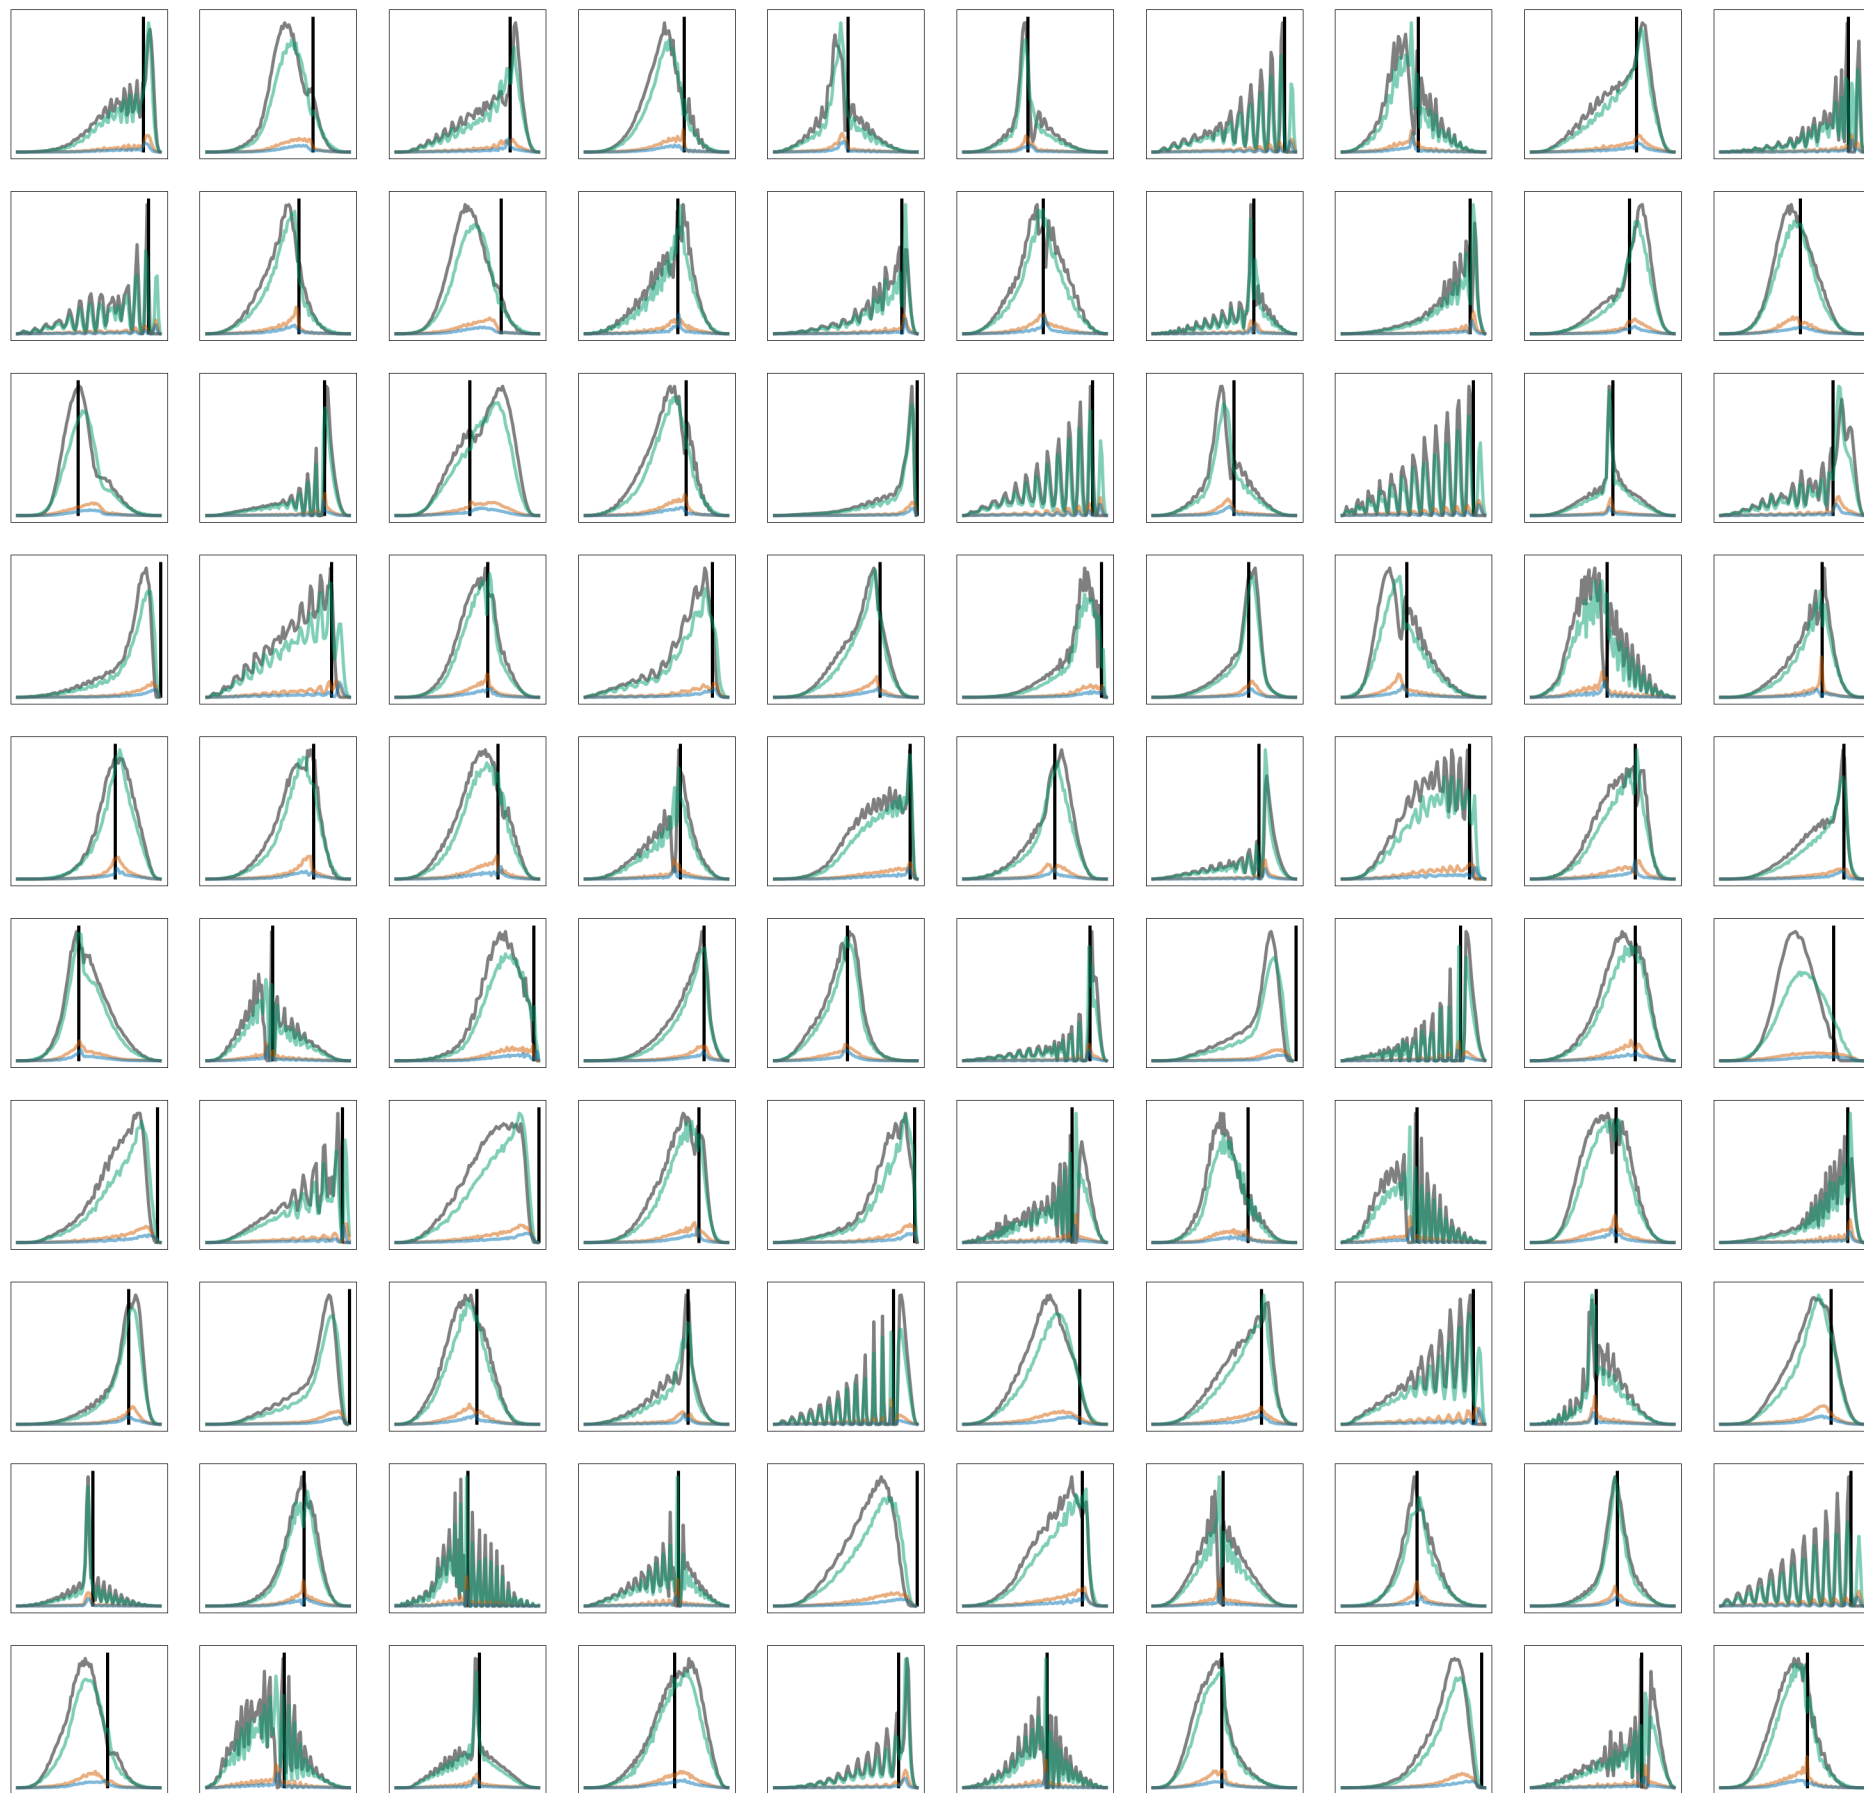

S3-compressnet-100-100-15-tuning-layer1

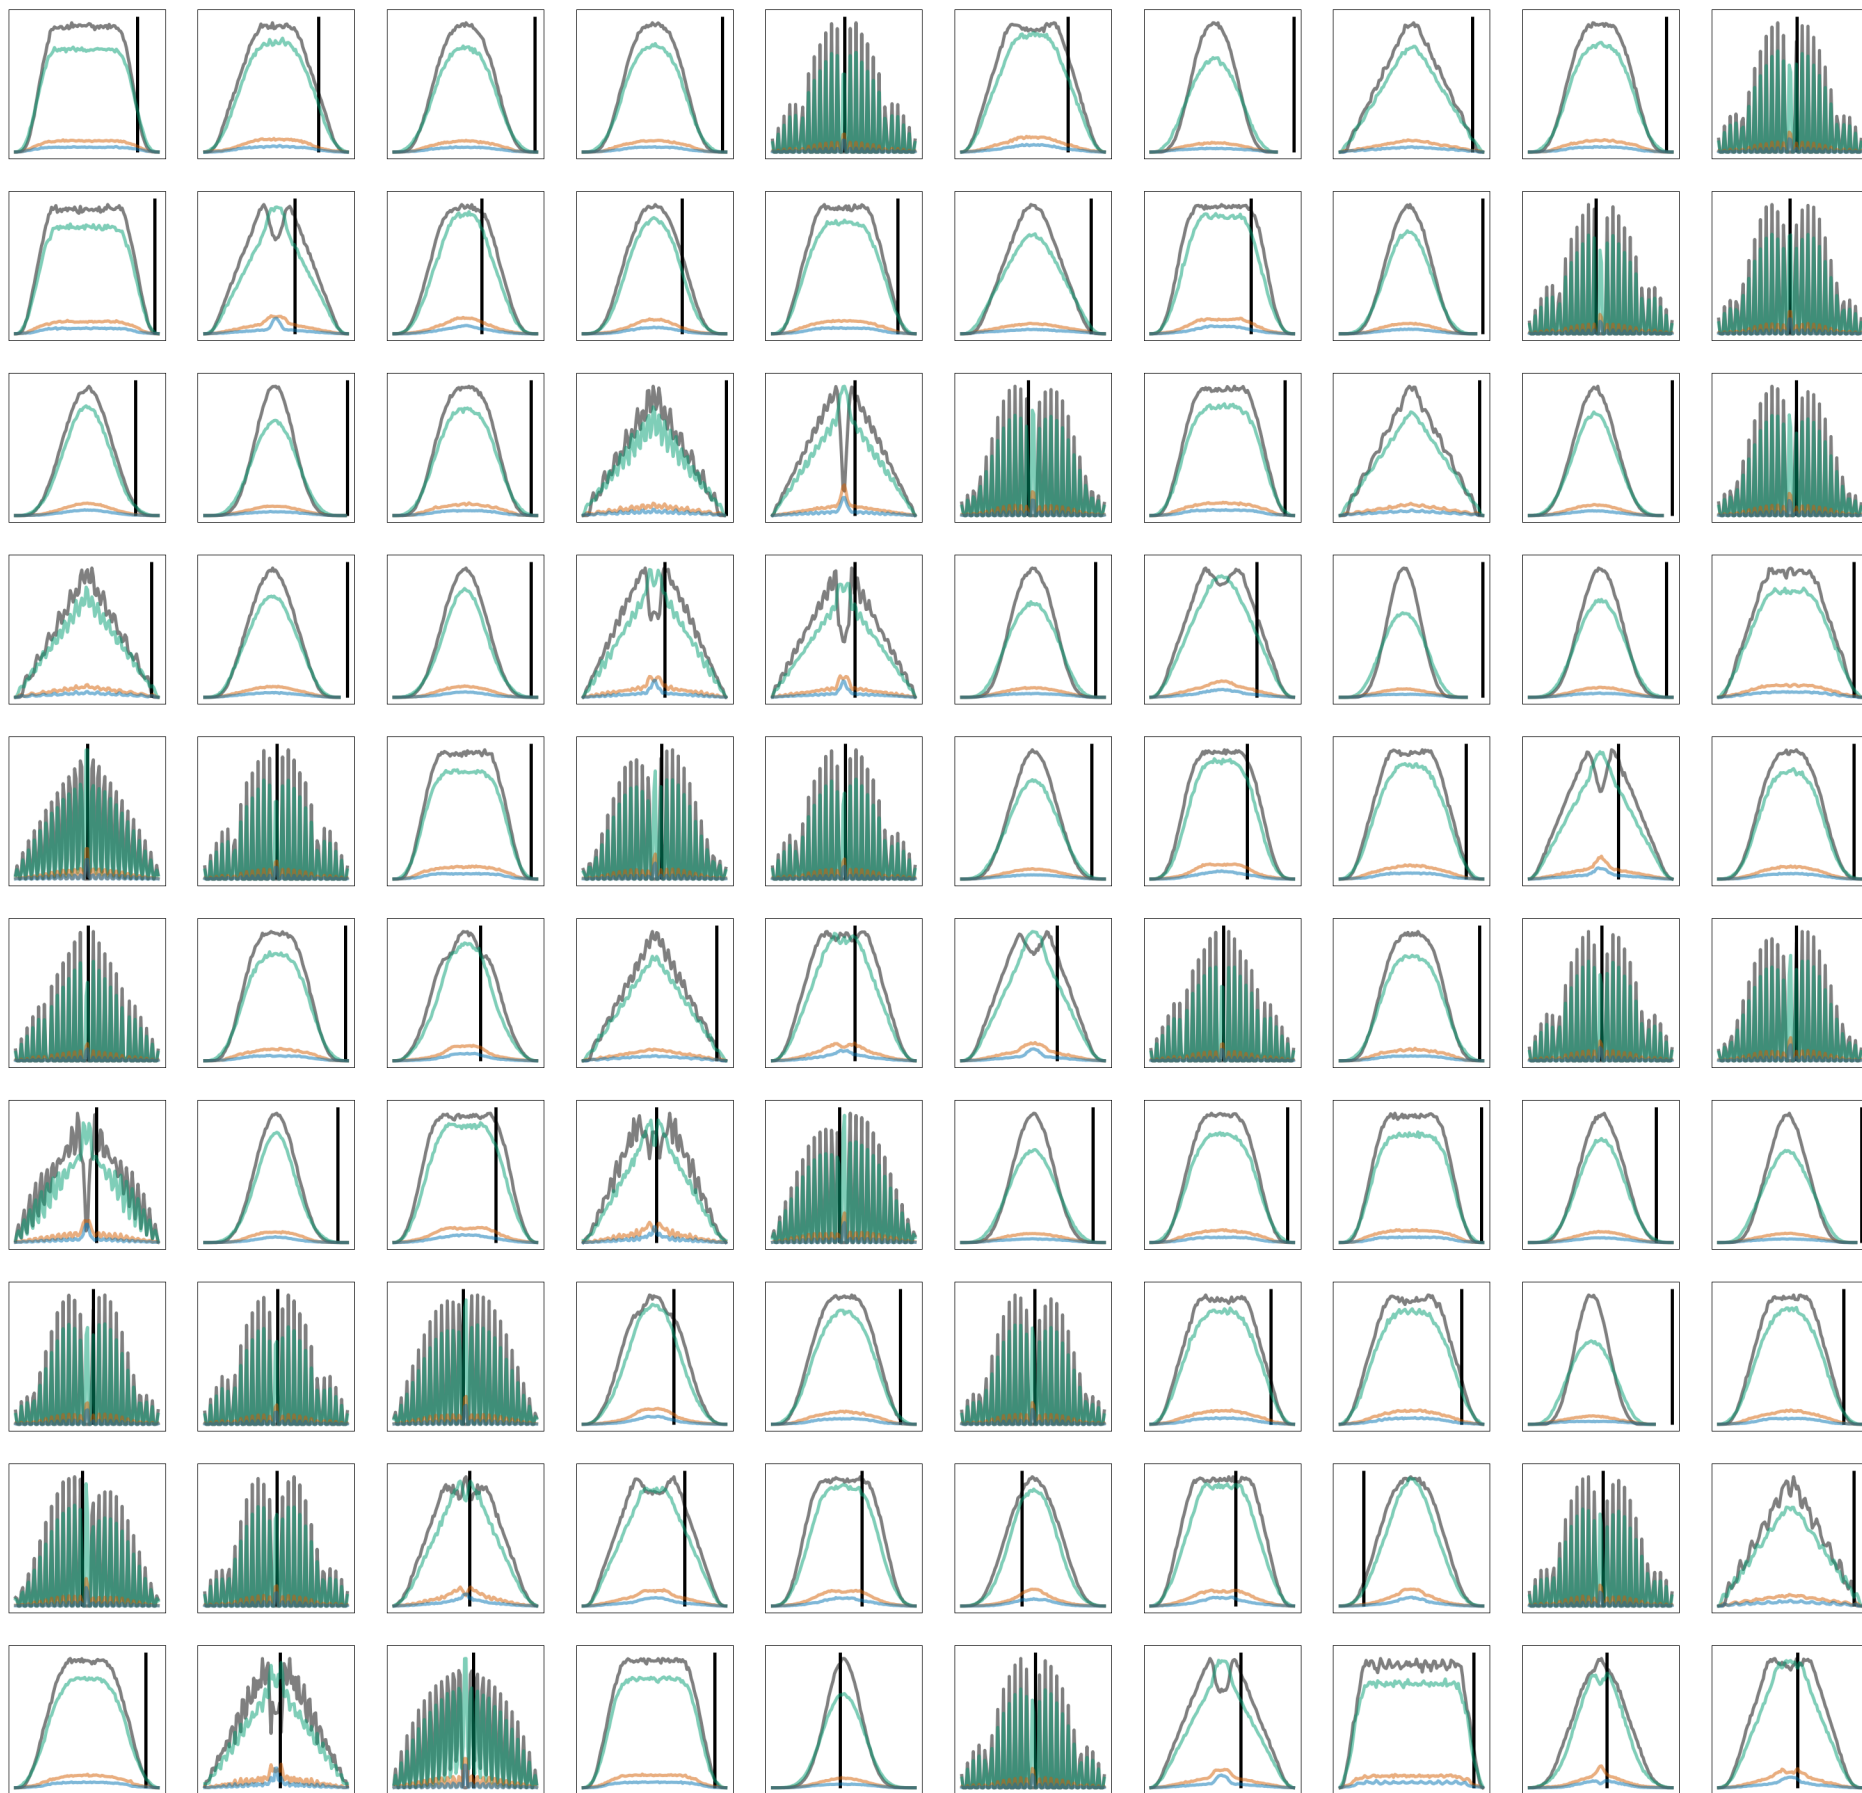

S4-compressnet-100-100-15-tuning-layer2

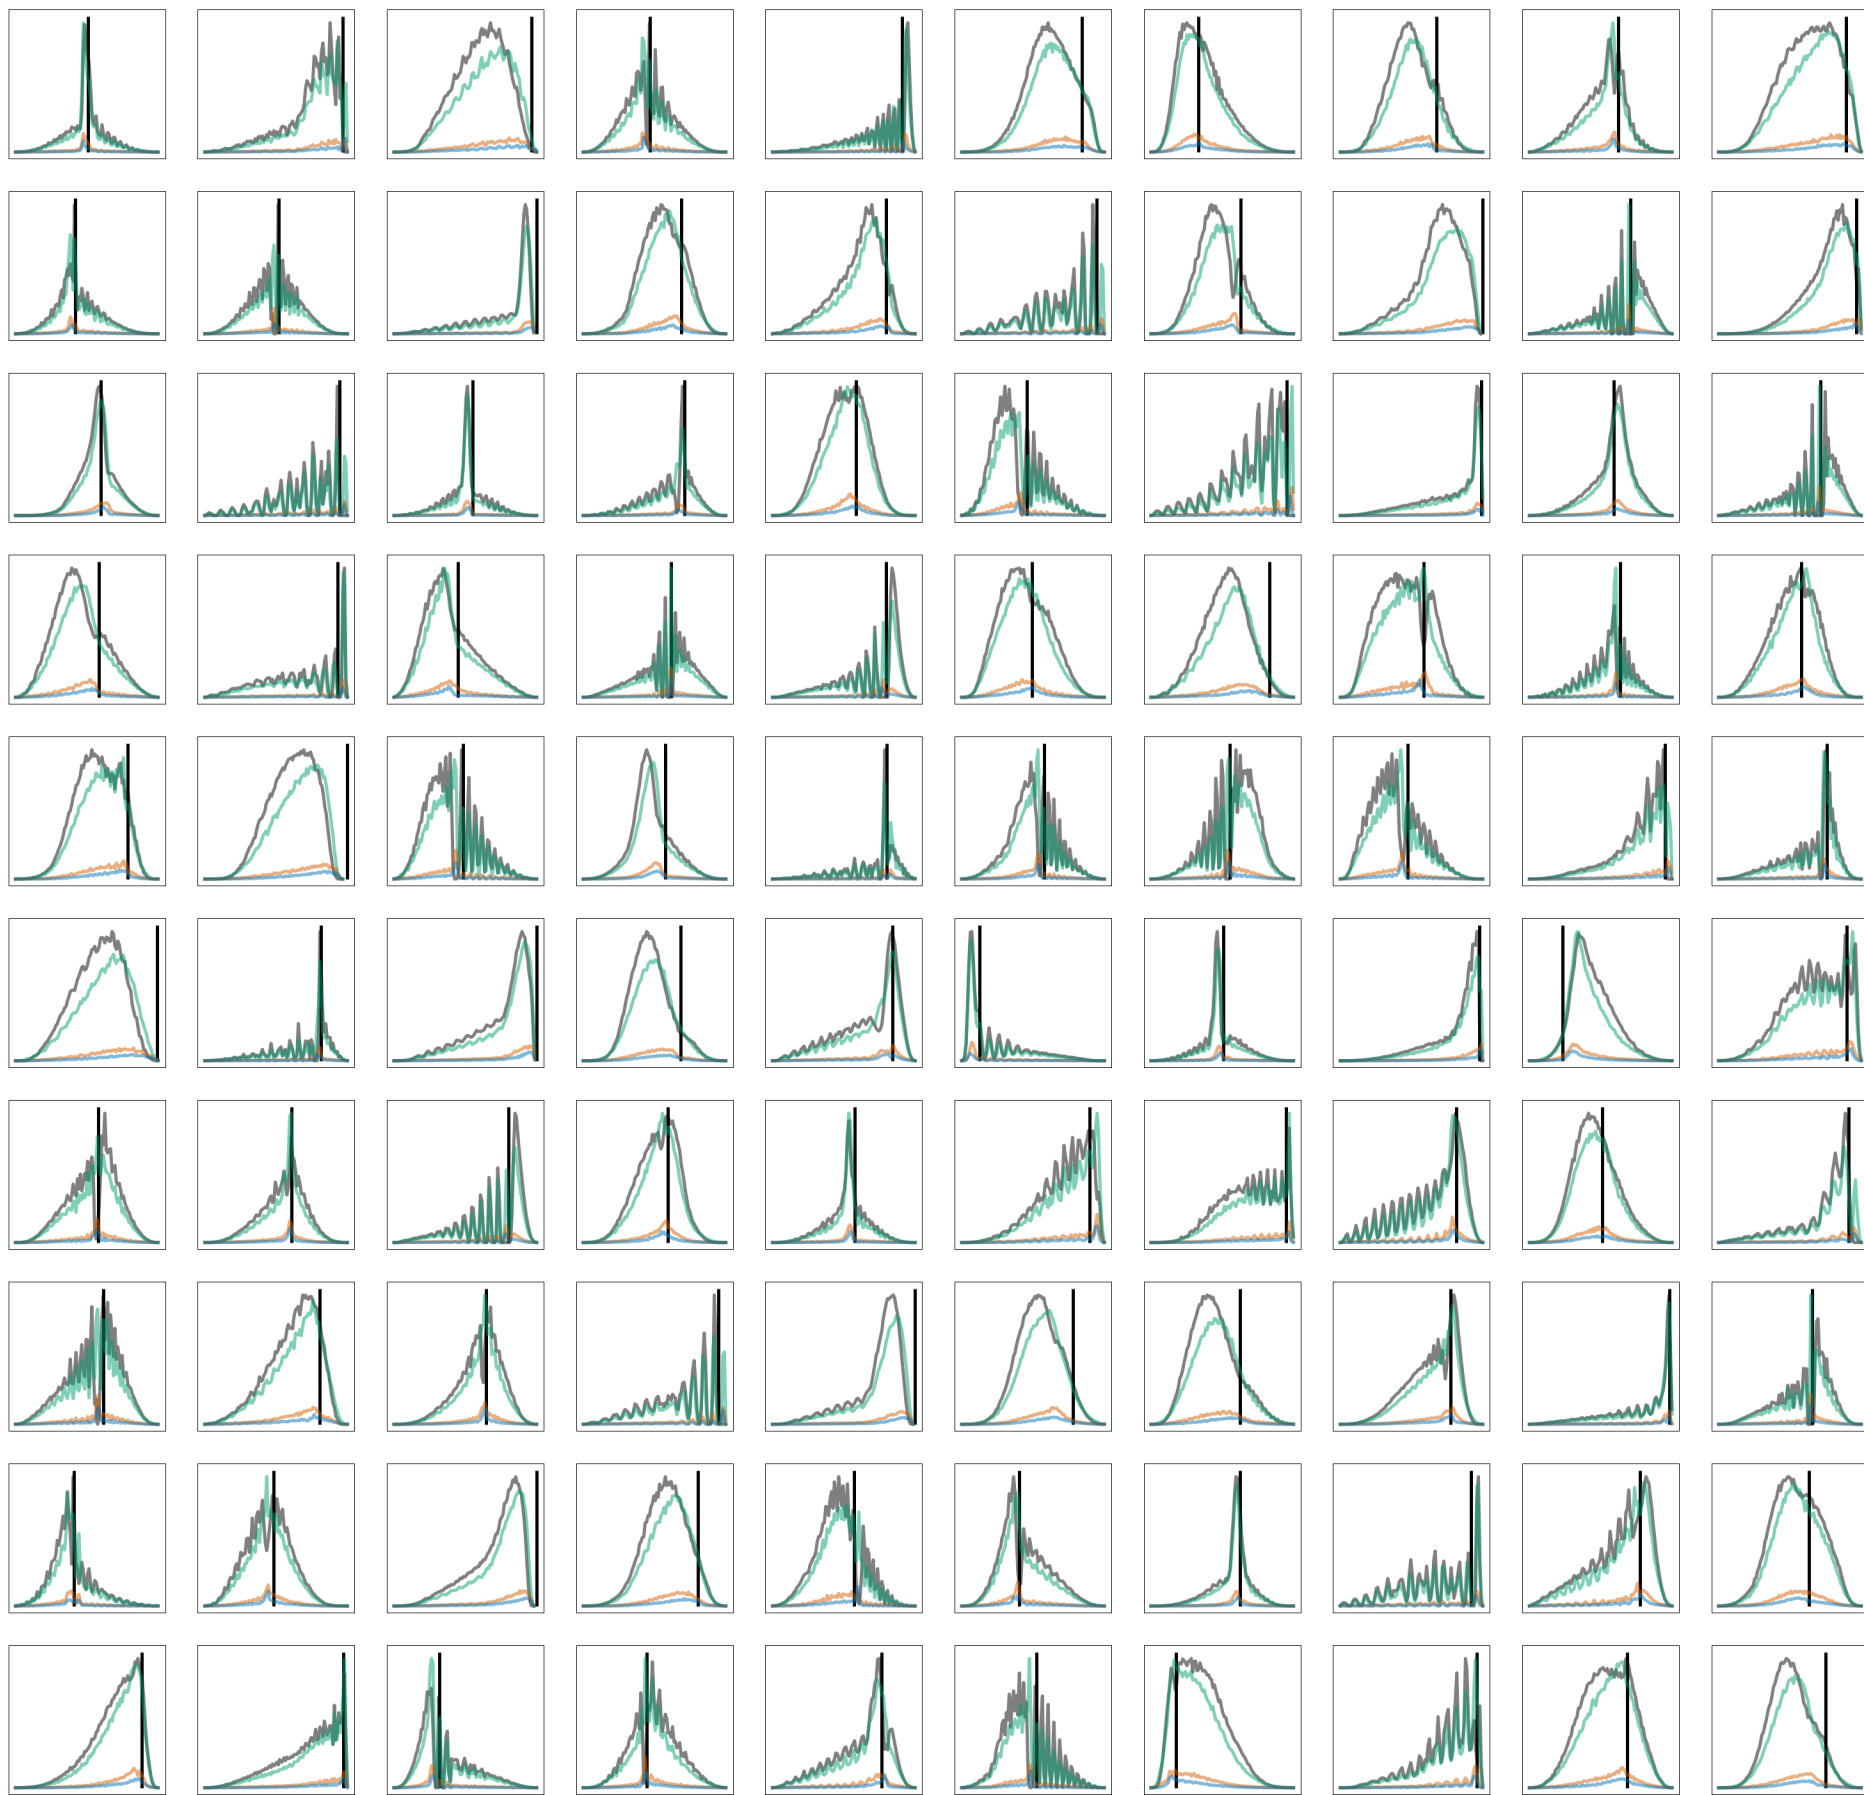

# S5-compressnet-100-100-15-tuning-layer3

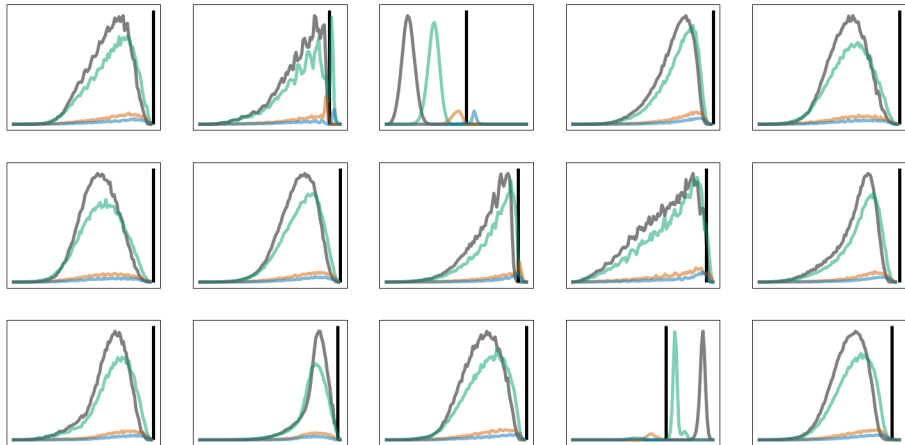



# S7-recurrent-trajectories-shearing-2deg

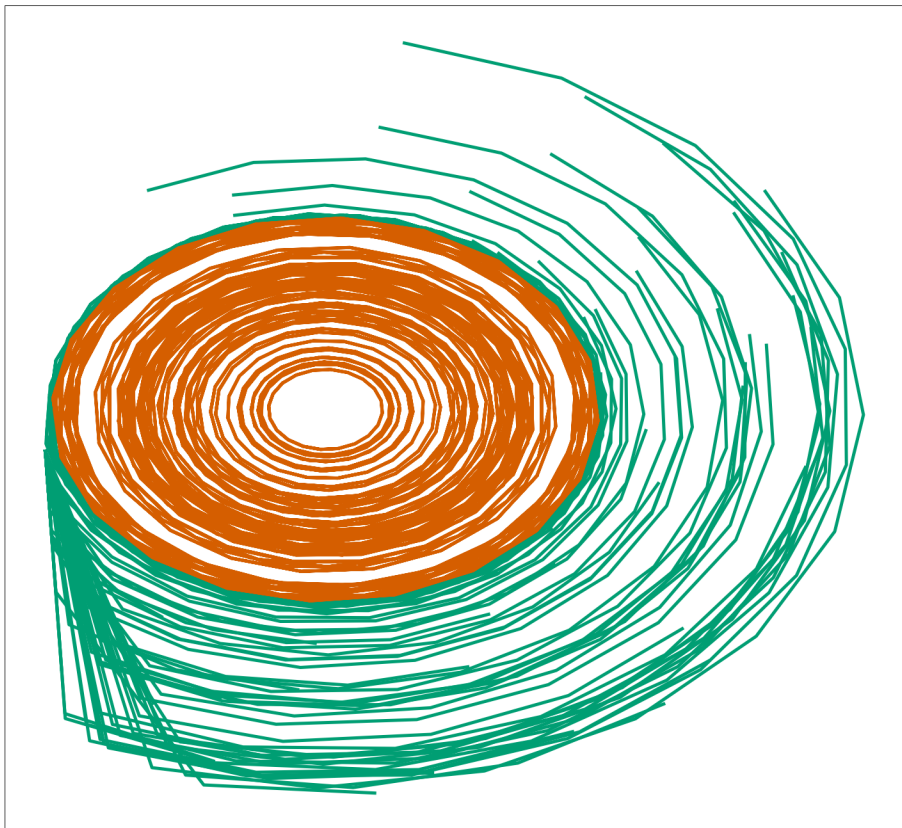

Supplement: Supplementary file 1 [file supplementary_figures.pdf]
